# Supplementary material for: CSP: A Simulator For Multi-Agent Ranking Competitions
Source: arXiv:2502.11197 source file (2025-02-16)
Supplement: Supplementary file 1 [file appendix.tex]

\appendix
\section{Platform synonyms}
\begin{table*}[htbp]
\caption{A glossary of terms used in {\platformName}.}
\centering

\resizebox{\textwidth}{!}{
\begin{tabular}{|p{2cm}|p{10cm}|}
\hline
\textbf{Field} & \textbf{Description} \\ 
\hline
game (gid) & A game consists of players competing against each other in a during a fixed number of rounds, and a fixed query and ranker. \\
\hline
competition & A competition comprises a batch of games, each predefined with a different query. \\
\hline
ranker & A function induces a ranking over a set of documents based on a given query that represents the information need. The ranker can be classical (e.g., Okapi) or neural (e.g., E5). \\
\hline
agent & An agent is an entity participating in a competition (i.e multiple games), characterized by properties such as its persona and its method of analyzing feedback from each round of a game. In our simulation, we focus on a specific class of LLM-based agents.  \\
\hline
player & A player is a specific instance of an agent participating in a particular game. \\
\hline
rank & The position of a document within a set of documents submitted by a group of players during a round of a game. \\
\hline
round & Single iteration within a game. In each round, the players analyzes the feedback from previous rounds and modify their candidate documents to aim for the highest ranking. \\
\hline
document id (docno) & An identifier for a document in the competition corpus, uniquely defined by the game (or query), round, and the player who authored the document. \\
\hline
document & A passage of fewer than 256 tokens that a player publishes in a round of a game. \\
\hline
group & A group is the set of players participating in a specific game. \\
\hline
winner & The winner is the player whose document is ranked first in a specific round of a game. \\
\hline
feedback & The rankings of all other players' documents in previous round(s) of the game. \\
\hline
query & Keywords that represent the information need. \\
\hline
query id (qid) & The identifier for a query. \\
\hline
\end{tabular}
}
\end{table*}
\section{Prompts of the LLM-based agents}\label{appendix_prompts}
In Figures \ref{prompt_system}, \ref{prompt_system_no_copy}, \ref{prompt_clean}, \ref{prompt_listwise}, and \ref{prompt_pairwise}, we present the prompts used for the LLM-based agents.
\begin{figure*}[t]
\centering
\input{prompts_and_confs/str_prompt_system}
\caption{System prompt for LLM-based agents. The system prompt includes instructions for the game and defines the agent's persona.}
\label{prompt_system}
\end{figure*}

\begin{figure*}[t]
\centering
\input{prompts_and_confs/str_system_no_copy}
\caption{System prompt for LLM-based agents with additional instruction for not copying as given to students in ranking competition \cite{nachimovsky_ranking-incentivized_2024}. The system prompt includes instructions for the game and defines the agent's persona.}
\label{prompt_system_no_copy}
\end{figure*}

\begin{figure*}[t]
\centering
\input{prompts_and_confs/str_prompt_clean}
\caption{Cleaning prompt submitted to the LLM to remove headers and prefixes from the generated text.}
\label{prompt_clean}
\end{figure*}

\begin{figure*}[t]
\centering
\input{prompts_and_confs/str_prompt_listwise}
\caption{Listwise user prompt used as feedback for an LLM-based agent. This user prompt includes feedback from the last two rounds. The most recent round presents documents from highest to lowest ranking in the group, excluding the current document: a, b, c, d. The second-to-last round presents documents from the entire group, ranked from highest to lowest: e, f, g, h, i.}
\label{prompt_listwise}
\end{figure*}

\begin{figure*}[t]
\centering
\input{prompts_and_confs/str_prompt_pairwise}
\caption{Pairwise user prompt used as feedback for an LLM-based agent. This user prompt includes feedback from the last three rounds. In each round, two documents (a,b), (c,d), (d,f) were randomly selected including their ranking r(a), r(b), r(c), r(d), r(e), r(f).}
\label{prompt_pairwise}
\end{figure*}

\section{{\platformName} code-base}\label{appendix_code-base}
\subsection{{\platformName} code-base and design}\label{appendix_code-base_design}
Our platform is built upon \textit{Python 3}, making it easy to install, and is composed of popular Python packages listed in a requirements file. We ensure adherence to Object-Oriented Programming (OOP) practices and include comments and logs to document the main steps during the execution of the simulation.

In Figure \ref{fig_flow} we present the flow of \platformName.
